# Supplementary material for: Quant-Arena: Benchmarking LLM Agents for Quantitative Trading Research
Source: arXiv:2610.30113 source file (2026-10-21)
Supplement: Supplementary file 1 [file 10_appendix_artifacts.tex]

\section{Experimental Records and Reproducibility}
\label{app:artifacts}

\subsection{Coverage and Representative Identifiers}

The accompanying \texttt{quant-arena-v1.zip} archive contains 76 representative runs: 38 iterative and 38 one-shot configurations across the supported effort levels. It includes 205 candidate records (180 completed and 25 failed), candidate source and feature specifications, 533 model-call records with retained redacted transcripts, and both evaluation windows for every frozen strategy. The saved outputs comprise 152 window-level metric records, 55,176 daily NAV rows, and daily stock-score arrays. The run records link candidate development to the evaluation of each committed strategy.

Table~\ref{tab:artifact_ids} identifies the 18 runs analyzed in the diagnostics (Sections~\ref{sec:signal}--\ref{sec:kepler}) and their committed candidates: for each model and setting, the run with the highest total score across efforts. Run identifiers have the form \texttt{stem-setting-effort}, where setting is \texttt{iterative} or \texttt{oneshot}. Candidate identifiers append \texttt{-c}$k$; $k$ is the submission index, including failed attempts, rather than the valid-candidate index in Figure~\ref{fig:progress}. Every one-shot run commits candidate \texttt{c1}.

\begin{table}[H]
\centering\small
\caption{Archive identifiers and provenance for the runs analyzed in the diagnostics. A: Arena generation and evaluation; S: standalone generation and standalone-harness evaluation. Generation and evaluation provenance are recorded separately.}
\label{tab:artifact_ids}
\setlength{\tabcolsep}{5pt}
\begin{tabular}{@{}llllll@{}}
\toprule
Run stem & Iter. effort & Iter. origin & Commit & One-shot effort & One-shot origin \\
\midrule
\texttt{astra-6} & xhigh & A & c5 & high & A \\
\texttt{sol-6} & xhigh & S & c5 & low & S \\
\texttt{terra-5.6} & max & A & c5 & none & A \\
\texttt{opus-5.5} & medium & A & c3 & medium & A \\
\texttt{gemini-3.8-flash} & medium & A & c3 & medium & A \\
\texttt{sonnet-5.5} & max & S & c2 & high & S \\
\texttt{glm-5.3} & max & A & c5 & high & A \\
\texttt{kimi-k3} & low & A & c5 & high & A \\
\texttt{deepseek-v4.1-flash} & low & A & c5 & max & A \\
\bottomrule
\end{tabular}
\end{table}

Across all 76 runs, 41 evaluations originate in the Arena and 35 in the standalone harness. Generation origins are 41 Arena, 29 standalone, and six frozen Arena strategies subsequently evaluated outside the platform. The six frozen strategies retain their original generation provenance. The reported representatives do not constitute a random sample of all historical attempts, and the records do not specify a selection rule over those attempts.

\subsection{Feedback, Budgets, and Accounting Axes}

Candidate \texttt{fb\_*} fields retain the legacy additive research metrics presented during iterative development. One-shot candidates have no performance-feedback values. The frozen-strategy metrics and NAV use cash-account evaluation. Figure~\ref{fig:progress} therefore reconstructs the feedback trajectory, while Table~\ref{tab:main} evaluates the committed strategy under the final financial conventions. The candidate trajectories thus describe the information available during development, while the final metrics describe the submitted strategies under common cash-account rules.

Token accounting is provider-reported for 74 runs and estimated for two. The Sonnet iterative max run records 566,294 tokens, exceeding the nominal 500,000-token target. Realized resource use is therefore heterogeneous, and comparisons across configurations should not be interpreted as strictly compute-matched.

NAV contains 484 research accounting dates and 242 sealed-period accounting dates. Saved signal arrays instead use their own labeled decision-session axes, with 483 and 241 sessions respectively, and include eligibility and session-presence masks. Signal analyses align observations by the labeled decision sessions and apply the eligibility and presence masks. Sessions with no finite scores are distinguished from absent observations.

\subsection{Numerical Consistency and Reproducibility Scope}

From the saved aggregate metrics and diversity counts, we reproduce all 76 public research-period scores with maximum absolute error below $2\times10^{-14}$. NAV terminal values reproduce all 152 reported ARRs under the archive's two documented precision conventions: saved terminal precision or terminal NAV rounded to six decimals. Saved daily drawdowns and headline MDD differ by less than $10^{-6}$ in return units. Recomputing the 36 sealed-period signal-correlation and Top-75 overlap pairs also recovers the summaries in Figure~\ref{fig:similarity}. These checks validate the numerical consistency of the saved outputs; they do not re-execute the strategies.

Independent reproduction of portfolio execution requires the underlying market observations, positions, and order or trade events in addition to the saved evaluation outputs. The numerical checks above cover scores, terminal returns, drawdowns, and signal similarity; the decile and holding-style figures are supplied diagnostics. Kepler-1 is evaluated through its headline scores and sealed-period metrics. Numerical consistency does not address historical pretraining exposure, representative selection, or repeated-run uncertainty.
