# Supplementary material for: Quant-Arena: Benchmarking LLM Agents for Quantitative Trading Research
Source: arXiv:2610.30113 source file (2026-10-21)
Supplement: Supplementary file 2 [file 7_appendix_boundary.tex]

\section{Information Boundary and Financial Evaluation Details}
\label{app:boundary}
\label{app:financial_details}

\subsection{Information Boundary}

The model conversation receives the public suite description, the platform documentation, the feedback permitted by the track, and its remaining budget. It never receives market data matrices, evaluation internals, or anything from the sealed window. Strategy code runs separately, with a market-data capability scoped to the permitted dates, stocks, and fields. A trusted supervisor holds that capability, so a strategy cannot widen its scope by requesting another date or forging credentials. The sealed window is served only to the final evaluator.

A commitment ends candidate selection. The same frozen strategy is used for the sealed assessment, and recovery after an interruption continues the recorded run without allowing a new candidate.

This boundary controls access at run time. It cannot rule out that historical market information appears in a model's pretraining data. A fixed historical sealed window is therefore a known limitation; refreshed sealed windows are a planned extension.

\subsection{Portfolio Diagnostics and Signal Metrics}

The main financial evaluation uses the portfolio specified in Section~\ref{sec:financial}. Top-200 and Top-400 portfolios provide supplementary diagnostics of how results depend on the breadth of stock selection. A common trading calendar is used to align the strategy's cash-account returns and the gross full-market equal-weight reference. Return and signal statistics use the annualization factor $N_{\mathrm{ann}}$ defined in Section~\ref{sec:financial}.

Daily RankIC is the cross-sectional rank correlation between stock scores and next-period returns. The reported RankIC is its mean over the evaluation window. Annualized RankICIR is the mean divided by the standard deviation of daily RankIC, multiplied by $\sqrt{N_{\mathrm{ann}}}$. Long--short Sharpe measures the return spread between the top and bottom score deciles. Turnover is the average daily replacement fraction of the main portfolio.

\subsection{Feature Diversity}
\label{app:diversity}

Diversity rewards strategies that combine several distinct sources of signal. A strategy may declare up to 300 named features. Features that pass a quality screen are grouped into clusters of highly correlated features. A cluster counts as \emph{used} if regressing the strategy's daily score ranks on the cluster's feature ranks shows a material unique contribution (threshold 0.01). $K$ is the number of used clusters. Duplicating a feature therefore adds nothing, and declaring a feature that the score ignores adds nothing. Clusters describe statistical redundancy, not distinct economic mechanisms. Equation~\eqref{eq:ed} normalizes $K$ by a fixed scale of 32 and caps $D$ at $Q$; this scale is independent of the declaration limit.

\subsection{Score Provenance}

The financial metrics and scores reported in this paper are recomputed offline from the recorded evaluations.
