# Supplementary material for: Quant-Arena: Benchmarking LLM Agents for Quantitative Trading Research
Source: arXiv:2610.30113 source file (2026-10-21)
Supplement: Supplementary file 3 [file 8_appendix_platform.tex]

\section{Arena Platform and Execution Records}
\label{app:platform}

The Arena separates model interaction, strategy computation, and trusted evaluation. The model-facing service exposes the objective, documentation, budget, and track-permitted feedback. A separate execution service runs the submitted program against authorized market history. The evaluator consumes daily scores and applies the common portfolio, accounting, and scoring rules. This separation allows data-intensive research without sending market-data matrices or sealed evaluation artifacts into the model conversation.

\subsection{Scoped Execution and Immutable Data}

A trusted supervisor controls data access and advances the strategy through authorized decision dates. Strategy processes receive date-, instrument-, and field-scoped capabilities and cannot expand that scope themselves. Research and sealed assessment use separately authorized executions. Accepted daily outputs and declared fitted artifacts provide the recorded state needed to continue an execution; the commitment fixes the program, environment, and declared features used in final assessment.

Market observations are bound to immutable publications with a fixed calendar and coverage specification. Queries resolve the publication authorized for the run. Updating a platform default does not redirect an active run to another data version. Consequently, a run's financial result must be interpreted together with its bound data release, temporal split, and evaluation conventions.

\subsection{Accounting and Recovery}

Model calls, research evaluations, and final commitments have persistent operation identities. Budget reservations are recorded separately from observed token consumption. Completed operations and accepted strategy outputs can be recovered after an interruption, preserving the original candidate history and remaining budget. An interruption does not authorize another candidate or reopen selection after commitment. If the outcome of a model operation is unresolved, recovery must reconcile that operation rather than silently replace it with another generation.

\subsection{Run Provenance}

A leaderboard record links the model and harness configuration, model calls, token observations, research evaluations, final commitment, and resulting scorecards. Failed and cancelled runs remain part of the platform record. The experimental snapshot in this paper reports one representative for each model--setting--effort configuration; its cross-model counts are not estimates of repeated-run uncertainty. Appendix~\ref{app:artifacts} links the main-table representatives to the accompanying archive, and Section~\ref{sec:scoring} specifies the public research-score calibration. Archive identifiers alone do not establish how representatives were selected from all historical attempts. A recorded trajectory supports inspection of what happened in that run, while new calls to an external model need not reproduce the same trajectory.
